# Supplementary material for: Experimental demonstration of superresolution of partially coherent light sources using parity sorting
Source: arXiv:2102.01603 ancillary file (2021-03-18)
Supplement: Supplementary file 1 [file Supplement_Superresolution_of_Partially_Coherent_Light_Using_Parity_Sorting.pdf]

# Supplementary Material : Experimental demonstration of superresolution of partially coherent light sources using parity sorting

S. A. Wadood,<sup>1,2</sup> Kevin Liang,<sup>1,2</sup> Yiyu Zhou,<sup>1,2</sup> Jing Yang,<sup>2,3</sup> M. A.  
Alonso,<sup>1,2,4</sup> X.-F. Qian,<sup>5</sup> T. Malhotra,<sup>2,3,\*</sup> S. M. Hashemi Rafsanjani,<sup>6</sup>  
Andrew N. Jordan,<sup>2,3,7</sup> Robert W. Boyd,<sup>1,2,3,8</sup> and A. N. Vamivakas<sup>1,2,3,9,†</sup>

<sup>1</sup>*The Institute of Optics, University of Rochester, Rochester, New York 14627, USA*

<sup>2</sup>*Center for Coherence and Quantum Optics,  
University of Rochester, Rochester, New York 14627, USA*

<sup>3</sup>*Department of Physics and Astronomy,  
University of Rochester, Rochester, New York 14627, USA*

<sup>4</sup>*Aix Marseille Univ, CNRS, Centrale Marseille,  
Institut Fresnel, UMR 7249, 13397 Marseille Cedex 20, France*

<sup>5</sup>*Department of Physics and Center for Quantum Science and Engineering,  
Stevens Institute of Technology, Hoboken, NJ 07030, USA*

<sup>6</sup>*Department of Physics, University of Miami, Coral Gables, Florida 33146, USA*

<sup>7</sup>*Institute for Quantum Studies, Chapman University, Orange, California 92866, USA*

<sup>8</sup>*Department of Physics, University of Ottawa,  
Ottawa, Ontario K1N 6N5, Canada*

<sup>9</sup>*Materials Science, University of Rochester, Rochester, NY 14627, USA*

## Abstract

This document provides supplementary information to ‘Experimental demonstration of super-resolution of partially coherent light sources using parity sorting’ by Wadood *et al.*

---

\* Currently with Facebook Reality Labs, Redmond, WA, USA

† [nick.vamivakas@rochester.edu](mailto:nick.vamivakas@rochester.edu)

## I. DERIVATION OF EQS. (2-3) OF THE MAIN TEXT

In this section, we derive Eqs. (2-3) of the main text. In the object plane, consider two monochromatic point source emitters separated by  $\delta$ , each emitting  $N_0$  photons. The degree of (spatial) coherence between the two sources is  $\gamma$ . In the Coherent Mode Decomposition (CMD), the cross-spectral density (CSD)  $W_O(x_1, x_2)$  at the object plane is given by

$$W_O(x_1, x_2) = 2N_0 \sum_{k=1}^2 p_k \phi_k^*(x_1) \phi_k(x_2), \quad (\text{S1})$$

where we assume  $p_1 + p_2 = 1$ ,  $p_1 - p_2 = \gamma$ ,  $p_{1,2} = (1 \pm \gamma)/2$ ,  $\phi_k(x) = f_+(x) - e^{ik\pi} f_-(x)$  are the symmetric ( $k=1$ ) and antisymmetric ( $k=2$ ) coherent modes. In the object plane,  $f_{\pm}(x) = \eta(x \pm \delta/2)$ , where  $\eta(x)$  are localized functions describing the point sources, and can be considered as regularized delta functions with a unit intensity integral, such that each source individually emits  $N_0$  photons. Equation (S1) shows that total object plane photon number  $\int dx W_O(x, x) = 2N_0(p_1 + p_2) = 2N_0$  is given by sum of intensities of the symmetric and antisymmetric modes. At the object plane, these coherent modes are orthogonal. In fact unitary propagation of the field preserves their orthogonal nature. However, the modes do not remain orthogonal after passing through the aperture of the imaging system, which is the fundamental cause of the loss of resolution.

Recall that the finite width of the point spread function (PSF) arises due to the nonunitary nature of the imaging system; the aperture behaves as a low pass filter, blocking photons of spatial frequencies higher than those determined by the system's numerical aperture [1]. Consider the canonical  $4f$  imaging system with a Gaussian aperture of width  $\sigma_{ap}$  at the Fourier plane. For simplicity, consider the lenses to be of infinite extent. Since the propagation up to the aperture is unitary, the number of photons hitting the aperture is  $2N_0$ . There are  $2N_0 p_1 = N_0(1 + \gamma)$  photons in the symmetric and  $2N_0 p_2 = N_0(1 - \gamma)$  photons in the antisymmetric mode hitting the aperture. At the aperture/Fourier plane, these modes behave like a cosine and sine, each with spatial frequency  $g = k\delta/2f$ , where  $k$  is the wavenumber and  $f$  is the focal length. For a large  $\delta$  such that  $\sigma_{ap}g \gg 1$ , the aperture samples many periods of the coherent modes. The aperture transmission is then a radiometric factor equal to the ratio  $\sigma_{ap}/\sigma_b$ , where  $\sigma_b$  is the beam width at the aperture. This factor is same for both the coherent modes in the limit  $\sigma_{ap}g \gg 1$ . As  $\delta$  becomes smaller such that  $\sigma_{ap}g \ll 1$ , the aperture samples less than a fringe period of the coherent modes.

This is the sub-Rayleigh regime of our interest. For the cosine modes, the aperture samples the peak of the fringe. For the sine modes, the aperture samples the fringe minimum. The smaller  $\delta$  gets, the transmission for the sine mode decreases, and the transmission for the cosine mode increases. The transmitted photons  $I_{1,2}$  for each mode are then given by

$$N_1 = \int dx \left( \frac{1}{8\pi\sigma_b^2} \right)^{1/2} 4 \cos^2(gx) e^{-\frac{x^2}{2\sigma_b^2}} e^{-\frac{x^2}{2\sigma_{ap}^2}} = 2N_0 p_1 \frac{\sigma_{ap}}{\sigma_b} \left( 1 + e^{-2g^2\sigma_{ap}^2} \right), \quad (\text{S2})$$

$$N_2 = \int dx \left( \frac{1}{8\pi\sigma_b^2} \right)^{1/2} 4 \sin^2(gx) e^{-\frac{x^2}{2\sigma_b^2}} e^{-\frac{x^2}{2\sigma_{ap}^2}} = 2N_0 p_2 \frac{\sigma_{ap}}{\sigma_b} \left( 1 - e^{-2g^2\sigma_{ap}^2} \right). \quad (\text{S3})$$

In deriving Eqs. (S19, S20), we have assumed the beam at the aperture is a cosine or sine times a broad Gaussian of width  $\sigma_b$  such that  $\sigma_b \gg \sigma_{ap}$ . Using  $p_1 + p_2 = 1$ , we find the total photons *transmitted* by the aperture is given by

$$N_t = N_1 + N_2 = 2N_0 \frac{\sigma_{ap}}{\sigma_b} \left( 1 + \gamma e^{-2g^2\sigma_{ap}^2} \right). \quad (\text{S4})$$

Eq. (S3) does not contradict energy conservation. The transmitted photon number  $I_1 + I_2$  is not a strictly conserved quantity since it is the photon number in a local (Gaussian-apodized) portion of a fringe pattern. In essence, Eq. (S3) simply shows that the aperture transmission depends on the spatial coherence among two partially coherent emitters.

The propagation from the aperture to the image plane is also unitary, and hence Eqs. (S2-S4) also give the number of symmetric, antisymmetric, and total image plane photons. At the image plane, the Gaussian PSF's width  $\sigma$  is related to  $\sigma_{ap}$  by  $k^2\sigma_{ap}^2/f^2 = 1/4\sigma^2$ . We then have, using  $g = k\delta/2f$ ,  $\exp[-2g^2\sigma_{ap}^2] = \exp[-\delta^2/8\sigma^2] = d$ , where  $d$  is the overlap integral of the Gaussian PSFs. The overlap is generated due to the nonunitary nature of the aperture, as is evident from our analysis. Finally, by substituting  $\kappa = \sigma_{ap}/\sigma_b$  and using  $p_{1,2} = (1 \pm \gamma)/2$ , Eqs. (S2-S4) reduce to Eqs. (2,3) of the manuscript.

## II. OFFLINE COHERENCE SYNTHESIS AND MODAL WEIGHTS VS. $\gamma$

In this section, we describe the offline coherence synthesis and measurements of the normalized image plane modal weights  $p_{1,2} = N_{1,2}/N_t$ , where  $N_t, N_{1,2}$  are given by Eqs. (2,3) of the main text.

Since we are working in the image plane model, we do not know  $N_0$  as explained in the Theory section of the text. For this section, we therefore denote the symmetric and

antisymmetric experimental photon numbers as  $N_{sym,asym}$  instead of  $N_{1,2}$  as used in Eq. (3) of the manuscript. Similarly, the total experimental image plane photon number is denoted as  $N_I = N_{sym} + N_{asym}$  instead of the theoretical  $N_t$  used in Eq. (2) of the manuscript. For a fixed  $\delta$ , we prepare an antisymmetric mode and record its photon number  $N_{asym}$  at the output of the parity sorter, which can be arbitrary but is dictated by experimental limitations such as phase noise of the interferometer, electronic noise and dynamic range of the detector etc. We then prepare a symmetric mode for the given  $\delta$ , and record its flux at the output of the parity sorter over a wide range of input powers. For a particular  $\gamma$  and  $\delta$ , the corresponding photon number  $N_{sym}$  of the symmetric mode is given as  $N_{sym} = KN_{asym}$ , where  $K = (1 + \gamma)(1 + d)/(1 - \gamma)(1 - d)$ . The modal weights are normalized by  $N_I$  such that  $p_{1,2} = N_{sym,asym}/(N_I)$ . We then post-select values for the desired  $\gamma$ . For example, assume  $\delta = 0.5\sigma$ , and 1 photon in the antisymmetric mode, i.e.,  $N_{asym} = 1$ . For  $N_{sym} = \{0, 10, 64, 100\}$  photons in the symmetric mode, the  $\gamma$  would correspond to  $\{-1, -0.72, 0, 0.2\}$  respectively. Note that the post-selected  $N_{sym}$  and  $N_{asym}$  are random variables which include both the quantum shot noise and the classical electronic and optical noise of the system. The post-selection is only applied to the ‘mean’ values of  $N_{asym}$  and  $N_{sym}$  satisfying  $\langle N_{sym} \rangle = K\langle N_{asym} \rangle$ , as explained in the section explaining the Image processing.

Figure (S1) shows the measured modal weights for different  $\gamma$  values. The solid red and blue lines in Fig. (S1a-c) are theoretically expected plots of odd and even modal weights respectively. The dashed lines are the theoretically expected plots incorporating effects of cross-talk. The circles indicate the mean values of data recorded for 10 measurements. For  $|\gamma| = 1$ , all the optical power is directed into a single port;  $P_1 = 1$  (solid red line) and  $P_2 = 0$  (solid blue line) for  $\gamma = 1$ . Similarly  $P_1 = 0$  and  $P_2 = 1$  for  $\gamma = -1$ . If the optical power in either port does not change as a function of  $\delta$ , which is the parameter to be estimated, one would expect no information to be gained by parity sorting. The error bars on all figures are too small to be visible on the graph. Finally, Fig. (S1 b) shows the modal weights measured for  $\gamma = -0.75$ . The modal weights change rapidly with  $\delta$ , and therefore one would expect a higher FI for  $\gamma = -0.75$  than for  $\gamma = 1, -1$ .

When processing the measured optical powers for the maximum likelihood estimation (MLE), we have subtracted any cross-talk, which was 8% on average, between the two ports. The cross-talk could be attributed to intensity mismatch of the two beams, finite coherence time, and fluctuations of path length and polarization in the two arms. This background

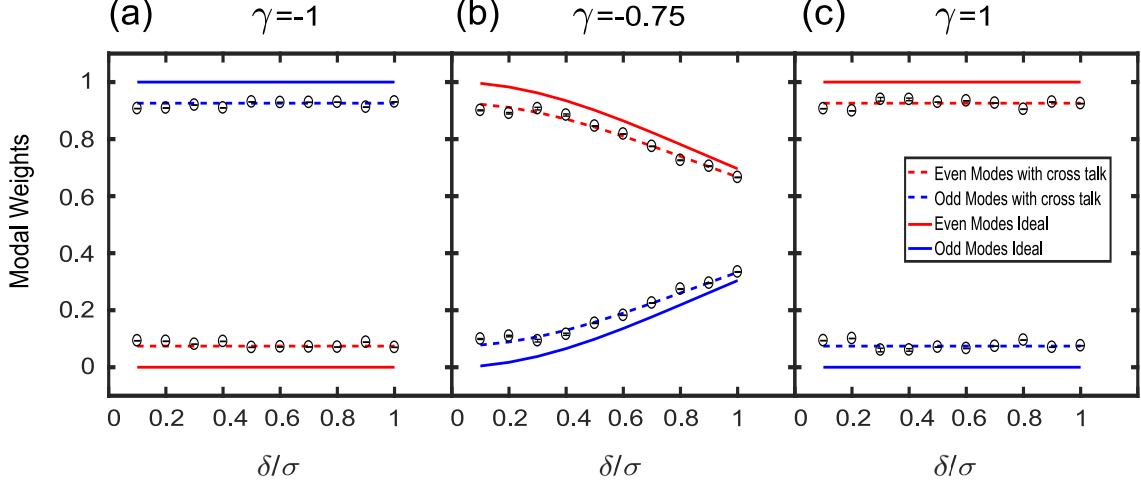

FIG. S1. Measured modal weights for the parity sorter. a-c: Modal weights for  $\gamma = -1, 1, -0.75$ . Blue and red color indicates the odd and even modal weights respectively. Solid lines indicate the theoretically expected modal weights with zero cross-talk. The dashed lines indicate the expected modal weights for 8% cross-talk. The circles indicate the measured values. All the modal weights are normalized by  $N_t$ , the total number of photons in the interferometer. Each point on the graphs represents a mean of 10 measurements, while the error bars are too small to be noticed on the graph. Note that for  $|\gamma| = 1$ , the modal weights are constant versus  $\delta$ .

subtraction is allowed because we are generating coherence offline by adding post-selected intensities, and only one of the coherent modes is present at a given time. Better alignment of the system can reduce the cross-talk. However, this experimental complexity is irrelevant to the analysis of partial coherence and thus is avoided in our proof-of-principle experiment by using offline coherence generation. Figure (S2) shows the cross-talk subtracted modal weights measured for  $\gamma = 0, \pm 0.25, \pm 0.5$ . Note that for a given  $\delta$ , the power in the symmetric (antisymmetric) mode increases (decreases) as  $\gamma$  becomes more positive.

### III. EXPERIMENTAL DETAILS

#### A. Mode Generation

The spatial light modulator (SLM) can be used to generate a field  $\psi(x, y)$  with an arbitrary transverse amplitude and phase profile. To that end, we implement a phase grating  $\exp[i(\Pi(x, y))]$  on the SLM. The grating is constrained such that the first-order term in its

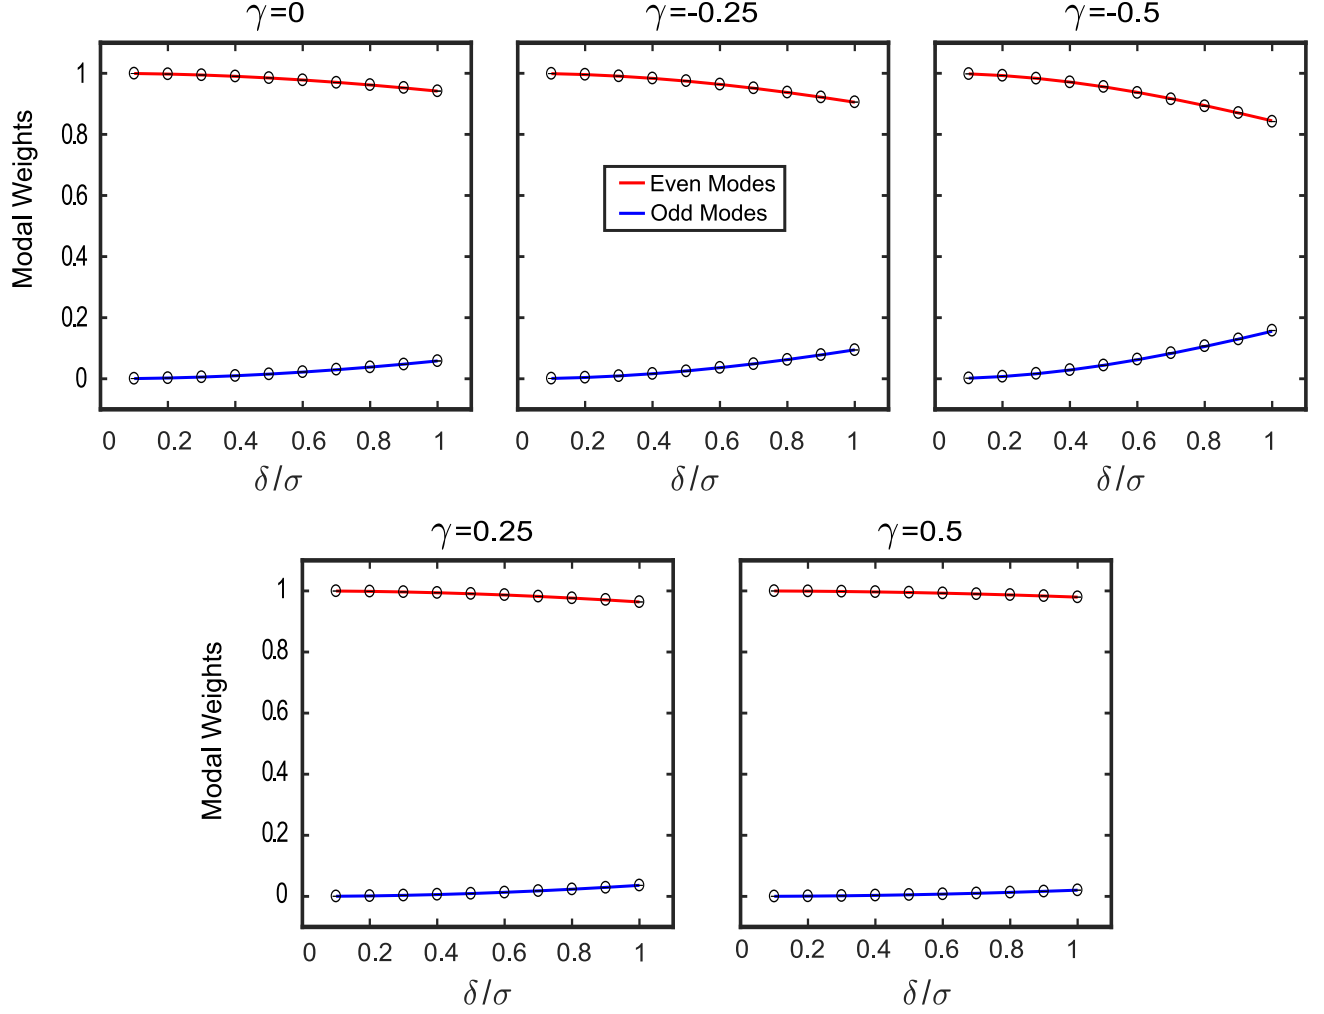

FIG. S2. Measured and expected modal weights for the parity sorter for  $\gamma = 0, \pm 0.25, \pm 0.5$ . Blue and red solid lines respectively indicate the theoretically expected modal weights for antisymmetric and symmetric mode. The circles indicate the measured modal weights. Each point on the graphs represents a mean of 10 measurements, while the error bars are too small to be noticed on the graph. Note that cross-talk has been subtracted for this data.

Fourier expansion equals  $\psi(x, y)$ . We add a linear phase grating and use a  $4f$  spatial filter to isolate the first diffraction order, which is proportional to  $\psi(x, y)$ . The details on the algorithm to ‘encode’ the field into the phase grating are given in [2]. Note that there are limits set on the spatial frequency content of the beams that can be generated. These limits are dictated primarily by the pixel pitch of the SLM, and the range of phase modulation that the liquid crystals can impart. The SLM model used in our experiment was HAMAMATSU X10468-02, which has a pixel pitch of  $20\mu m$  and phase modulation range of  $2\pi$ . Due to the

small pixel pitch, any discretization effects are negligible in our experiment. The SLM only responds to a horizontally polarized beam (polarization axis parallel to the optical table).

Figure (S S3a) shows the SLM and the  $4f$  spatial filter that filters the desired beam. Figure (S S3b) shows the phase grating implemented on the SLM to generate the coherent modes. The high spatial frequency fringes show the linear grating implemented to separate the desired mode on the first diffraction order. Note that the phase mask is qualitatively very similar to the beam itself. The beam is relayed to the interferometer with  $4f$  systems.

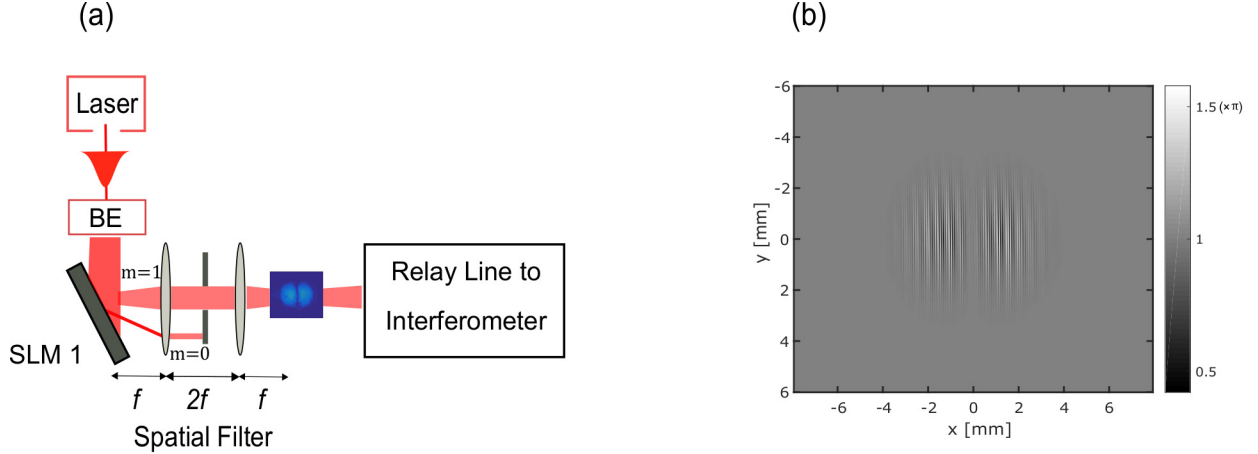

FIG. S3. a: Generation of Coherent Modes: A 795 nm linearly polarized Gaussian beam passes through a beam expander (BE) and is then transformed into one of the coherent modes, via a mode converter consisting of a phase SLM and a spatial filtering setup, which selects the  $m = 1$  diffraction order. Polarization optics and attenuators, not shown, are used to control the power of the beam. The beam is relayed to the interferometer with  $4f$  systems. b: Phase mask implemented on the SLM to generate the antisymmetric mode with  $\delta/\sigma = 0.2$ . The high spatial frequency tilt fringes form the grating that routes the desired mode into the first diffraction order shown in (a).

## B. Parity Sorter Details

The basic schematic of the parity sorter is given in Fig. (2) of the main text. Here we give details of the implementation of the  $2f$  arm of the interferometer. A horizontally polarized beam (polarization parallel to the optical table) is used for the parity sorting. Fig. (S4) shows the  $2f$  arm having 2 SLMs separated by a distance of 600mm. SLM 2 has a focal length of 600 mm and SLM 3 a focal length of 300 mm. The optical power on SLM 2

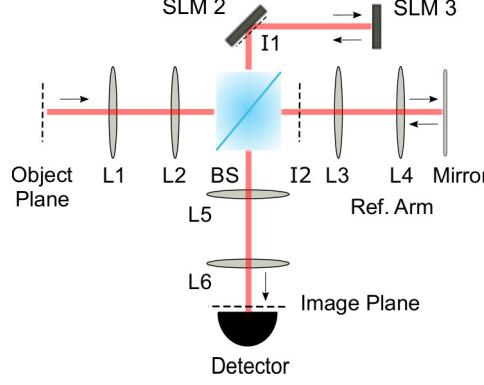

FIG. S4. Parity Sorter. An input beam is split at the beamsplitter. In one arm, the two SLMs form a  $2f$  system with SLM 2 having a focal length of 600 mm, SLM 3 having a focal length of 300 mm, and the distance between the two SLMs equal to 600 mm. The transformed beam interferes with the untransformed beam that goes through the reference arm. The interference pattern is detected at the output with a CCD to take images or with a bucket detector to measure total power. Throughout the interferometer, we use  $4f$  relay systems to avoid any diffraction-induced phase. The input  $4f$  relays the beam from the coherent mode generation part of the setup with unit magnification ( $f_{L1}, f_{L2} = 200$  mm). The  $4f$  in the reference arm has a magnification of 0.5 ( $f_{L3} = 200$  mm,  $f_{L2} = 100$  mm) (double pass magnification is unity). The final  $4f$  system in the output arm relays to the bucket detector the field at SLM 2 and the reference arm field with a 0.5 magnification factor ( $f_{L5} = 200$  mm,  $f_{L6} = 100$  mm).  $I1, I2$  denote the intermediate image planes in the SLM and reference arms respectively. BS: Beamsplitter, Ref. arm: Reference arm.

cancels the quadratic phase at the image plane of SLM 3, which coincides with the SLM 2 plane. The interferometer is path stabilized using a PID loop connected to the reference arm mirror. To monitor the phase fluctuations for the PID loop, a separate vertically polarized beam (not shown in Fig. (S4)) is sent to the interferometer, separated before the detector via a polarizing beam splitter, and its measured power is fed to the PID loop. Note that the SLMs do not respond to the vertically polarized beam. The global phase difference  $\theta$  between the two arms for the signal beam is also implemented on SLM 2. For  $\theta = 0, \pi$ , the parity sorter respectively routes the even and odd modes to the detector port.

### C. Mode Intensity vs. $\delta$

In our superresolution experiment, we directly prepare the object plane field represented by Eq. (S1) through the SLM and subsequent offline addition of modes. Specifically, this technique allows us to avoid the more complicated procedure of preparing two actual emitters with varying  $\gamma$  and  $\delta$  and a physical Gaussian aperture whose transmission varies according to Eq. (S21). To this end, the power in the coherent modes does not depend on  $\delta$ . This is because the SLM is fundamentally a phase grating whose first diffraction order contains the desired coherent mode. Ideally, the efficiency of the grating is independent of  $\delta$ , except for the zero-photon case of  $\gamma = -1$  and  $\delta = 0$  in which case no grating phase is implemented. As long as the SLM pixel pitch and phase modulation range are not the bottleneck for a given phase grating, the grating efficiency and hence the power in a mode will not change with  $\delta$ . Figure (S S5) shows the power in the symmetric and antisymmetric modes measured for a fixed input power incident on the SLM. We see that the mode power is independent of  $\delta$ . The grating efficiency for the symmetric mode is actually lower than the antisymmetric mode, which causes the lower power in the symmetric mode. We can control the power going to the interferometer with polarization optics, and can equate the powers of the mode *after* the SLM.

### D. Image Processing

The basic idea of coherent mode decomposition (CMD) is to add the symmetric and antisymmetric modes on an intensity basis. For a specific  $\delta$  and  $\gamma$ , the relative intensity of the symmetric and antisymmetric mode is  $p_1/p_2 = K + (1 + \gamma)(1 + d)/(1 - \gamma)(1 - d)$  as evident from Eqs. (3) in the manuscript. For example, if  $\gamma = 0$  and  $(\delta/\sigma)^2 = -8\ln[0.5]$  such that  $d = 0.5$ , then  $p_1/p_2 = 3$ . To ‘prepare’ the  $\gamma = 0$  intensity offline for this  $\delta$ , one then needs to have a symmetric mode with thrice the power of the antisymmetric mode. As will be explained below, we post-select the required powers for each coherent mode from an array of recorded powers. These post-selected powers are then used to obtain the ML estimate  $\hat{\delta}$ . This process is repeated 100 times and the variance  $\text{Var}[\hat{\delta}]$  is then compared with the CRB.

We measure  $\text{Var}[\hat{\delta}]$  for  $\gamma = 0$  and  $\gamma = -0.75$ . For these  $\gamma$  values and  $\delta/\sigma < 1$ , the power

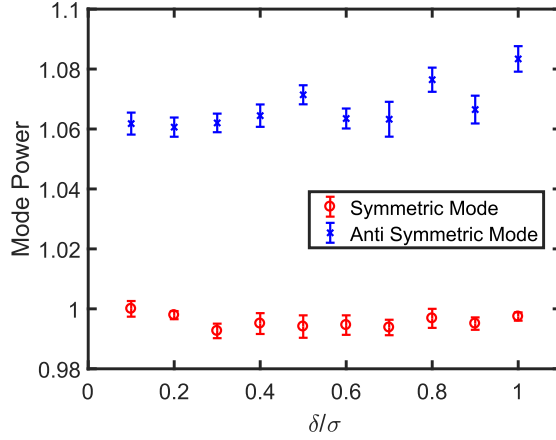

FIG. S5. Power in the Coherent modes versus  $\delta$  for fixed input laser power impinging on the SLM. The power has been normalized to the power in the Symmetric mode for  $\delta = 0.1\sigma$ . Note that the power in the antisymmetric mode is consistently higher because the higher diffraction efficiency of the SLM phase grating required to generate the antisymmetric mode. Ten images were taken for each data point.

in the symmetric mode is always larger than the power in the antisymmetric modes, as is evident from Figs. (S1, S2). Therefore, a large dynamic range is required to accurately measure these modal weights. To increase the dynamic range of our measured powers, we use the fact that our problem is 1D ( $x$  dimension), while the coherent mode is 2D; the coherent modes are a symmetric zeroth order Gaussian in  $y$ . The integrated power in each row of the coherent mode then corresponds to an independent parity sorting measurement.  $N$  rows in the mode then correspond to  $N$  bucket detectors performing parity sorting measurements. Figure (S6) shows the an image of the coherent modes for  $\delta = 0.4\sigma$  and the marginals. Specifically, each point on the Y marginal is used as an independent realization of a parity sorting measurement. This is allowed because we are using an approximately single-mode laser source, for which the pixels on the CCD are uncorrelated in intensity [3]. It is from these Y marginals of the symmetric and antisymmetric modes that we choose the photon numbers  $N_{sym,asym}$  such that  $N_{sym} = KN_{asym}$ .

To saturate the Cramer–Rao bound (CRB), the system should be shot-noise limited. This means that the photon numbers used from the Y marginals should have Poisson statistics. We choose a low noise Gigajot CCD with a dark current of less than  $0.5\text{ e}^-/\text{s}/\text{pixel}$  at room temperature [4]. The photoelectron statistics of each arm of the interferometer

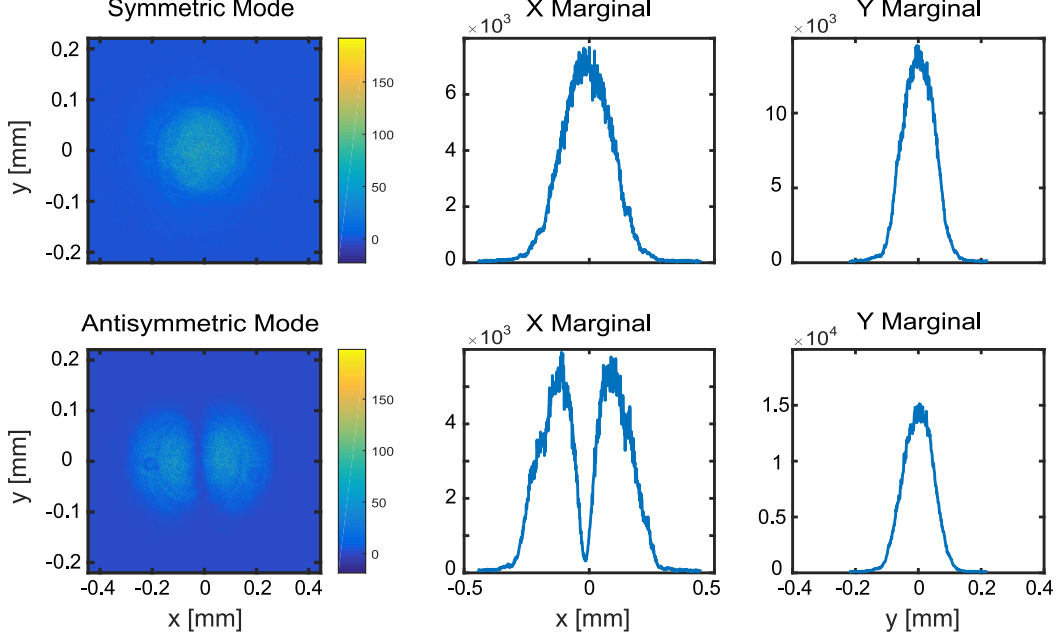

FIG. S6. Sample Image of Coherent Modes and their marginals for  $\delta = 0.4\sigma$ . Each pixel value on the Y marginal is counted as a bucket detector output in the parity sorter. The colorbar on the mode images and the y-axis on the marginals represent the detected photoelectron number.

are shot noise limited, as can be found by blocking the other arm. We show the noise statistics of the interferometer output in Fig. (S7). For every pixel on the Y marginal, we have three numbers: (i) the mean intensity  $\langle I(y) \rangle$  (circles and solid blue line), where  $I(y) = \int dx |\phi(x, y)|^2$  is the integrated intensity across  $x$  and the ensemble average is taken across the 100 acquired images. (ii) The variance  $\langle \Delta I^2(y) \rangle = \langle I^2(y) \rangle - \langle I(y) \rangle^2$  (solid orange line), and (iii) the noise metric  $M(y) = (\langle \Delta I^2(y) \rangle - \langle I(y) \rangle) / \langle I(y) \rangle$  (cross and solid purple line).  $M \approx 0$  corresponds to shot noise statistics, while any classical (electronic or optical) fluctuations will increase the value of  $M$ . In Fig. (S7), the reference arm statistics shows that the centre portion of the Y marginal Gaussian is close to being shot noise limited because of the high intensity, as opposed to the tails of the Gaussian. In contrast, the interference images, for which both arms are unblocked, have high  $M$  values in the centre of the Gaussian. Note that the classical noise is more pronounced in the antisymmetric mode compared to the symmetric mode.

The major noise source in our interferometer is phase noise due to path length fluctuations in the interferometer. Moreover, the phase noise fluctuations do not affect the coherent modes globally. This is due to the mode inhomogeneities introduced due to phase jumps in

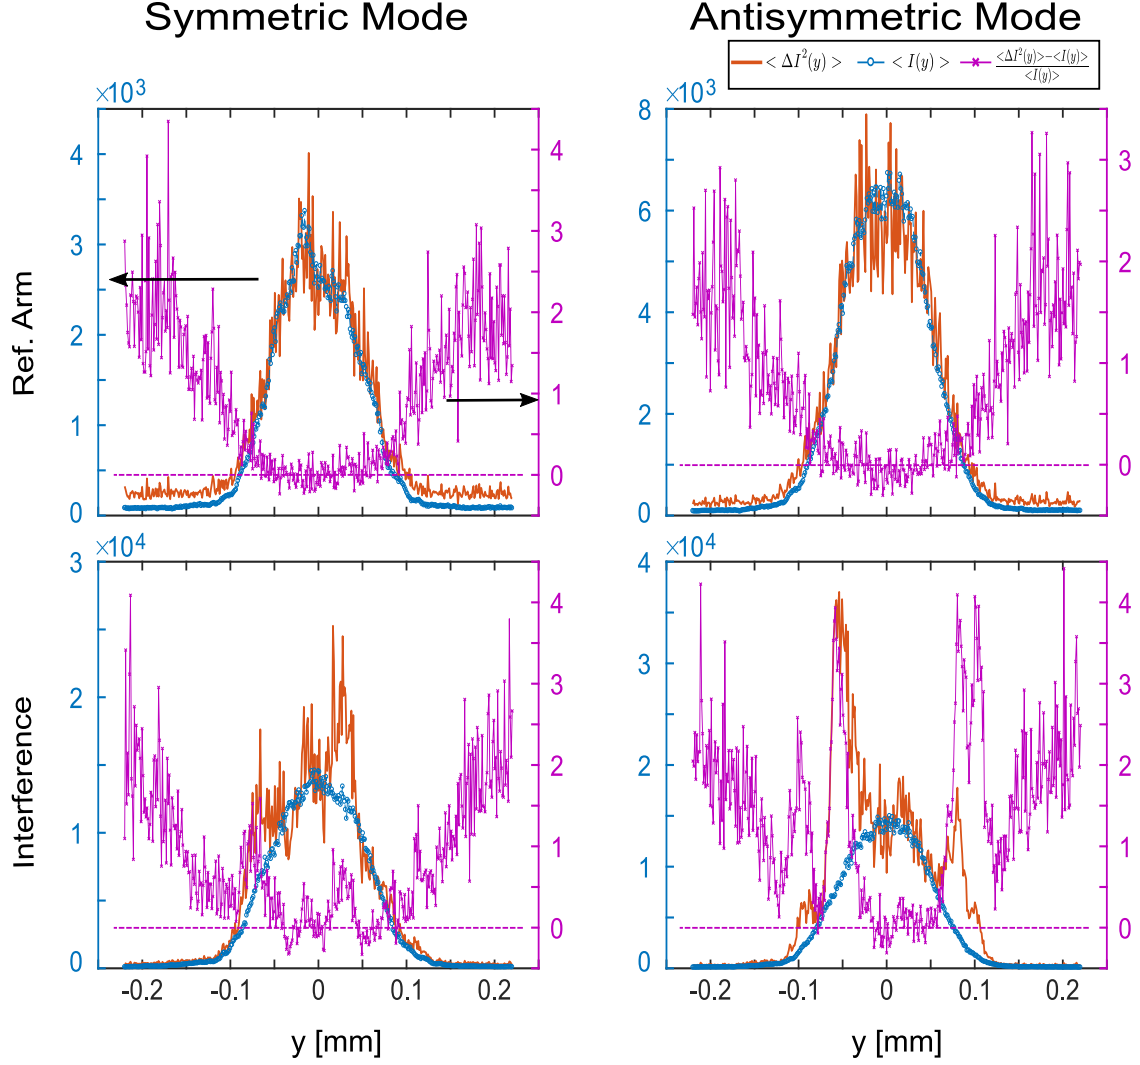

FIG. S7. Noise statistics of the parity sorter. All figures show the statistics of the Y marginal. Top row shows the statistics of the reference arm, with the  $2f$  imaging SLM arm blocked. Bottom row shows the statistics of the interference images, with both arms unblocked. Solid blue lines and circles represent the mean value  $\langle I(y) \rangle$  over 100 images (blue y-axis on left). Solid orange line represents the variance  $\langle \Delta I^2(y) \rangle$ . Solid purple line and crosses represent the noise metric  $M(y)$  (purple y-axis on right). The dashed purple line represents the shot noise limit  $M = 0$ . Note that the two reference and interference images were taken separately with different laser powers, so the reference image power is not exactly half that of the interference image power. The text discusses details of the figure.

the SLM arm of the interferometer [5] that implements the  $2f$  system. The peaks in the noise of the interference images in Fig. (S7) are due to the mode inhomogeneities caused mainly due to phase rings of the SLM coupled with the path length fluctuations. However, there is a significant number of rows that are relatively less affected by phase fluctuations such that  $M(y) < 1$ . These are the rows we use in the ML estimator. We sort the rows in ascending order according to the metric  $M(y)$ , and use these sorted rows in the CMD; rows with the lowest absolute  $M(y)$  value is picked first for CMD. Note that  $M(y) < 0$  is possible because of the finite size of our ensemble of 100 images, and we therefore sort based on  $|M(y)|$  rather than  $M(y)$ . A consequence of our CMD algorithm is that data for a higher  $\gamma$  will have a higher photon number. This is because for a higher  $\gamma$  on the real line, the ratio  $p_1/p_2$  increases as  $1/(1 - \gamma)$ , and hence we require more rows of the symmetric mode to generate the required coherent mode power. Another effect of this algorithm is that data for a higher  $\gamma$  will have higher (classical) noise, since more rows are added. The difference in the noise due to the different number of rows is observed to be not significant, however, in our experiment. One way to mitigate this noise difference is to take more images and add them to equal a 100 images. This will decrease phase fluctuations due to averaging. For  $\delta = 0.2 - 0.5$ , we took [500 - 200] images and added them together to prepare 100 images each for processing. In Fig. (3) of the manuscript, we compare  $\gamma = 0$  and  $\gamma = -0.75$ , for which the number of rows do not differ significantly and hence the phase noise is approximately the same for both  $\gamma$  cases.

### E. Photon number in Fig. (3) of Main text

Figure (3b) of the main text compares the product of the mean squared error ( $\text{MSE}/4\sigma^2$ ) and the mean total image plane photon number ( $N_I$ ) used for each iteration in the 100 estimates. This was done because the CRB lowerbounds the product  $N_I \text{Var}[\hat{\delta}]$  and not just  $\text{Var}[\hat{\delta}]$ . It is still instructive to look at the actual photon number and the mean squared error separately. As explained in the Image Processing section, the mean photon number is not the same for  $\gamma = 0$  and  $\gamma = -0.75$ . In Fig. (S8) we show the actual values of the photon number and the mean squared error, i.e.,  $\text{Var}[\hat{\delta}]$  for both  $\gamma = 0, -0.75$ . Note that the photon number for  $\gamma = 0$  is consistently *higher* than the photon number for  $\gamma = -0.75$ . Despite that, because the FI for  $\gamma = -0.75$  is higher than the FI for  $\gamma = 0$  case, the variance

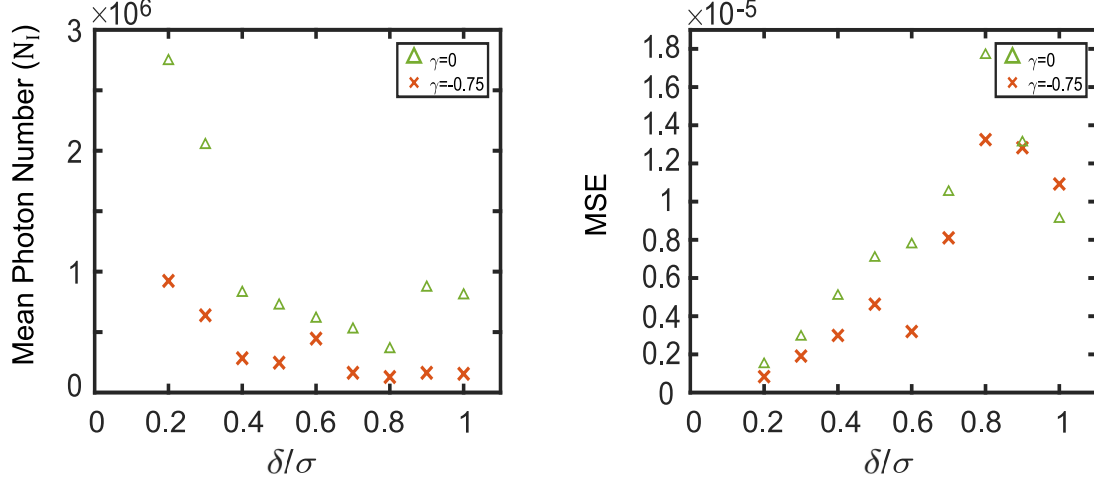

FIG. S8. Left: Mean total image plane photon number  $N_I$  per iteration used in estimation of  $\delta$ . Note that the photon number for  $\gamma = 0$  (green triangles) is consistently higher than the photon number for  $\gamma = -0.75$ . Right: The MSE for  $\gamma = 0, -0.75$ . The MSE for  $\gamma = -0.75$  is consistently less than the MSE for the  $\gamma = 0$  case.

for partially anticorrelated case is always *lower* than the variance for the incoherent case. Had the photon number in the  $\gamma = -0.75$  case been increased to match the  $\gamma = 0$  photon number, the variance in the  $\gamma = -0.75$  case would have dropped even further. This shows unambiguously that for the same number of photons, partial anticorrelation among the sources leads to a lower variance than the incoherent scenario.

- 
- [1] J. W. Goodman, *Introduction to Fourier Optics* (Roberts and Company Publishers, 2005).
  - [2] V. Arrizón, U. Ruiz, R. Carrada, and L. A. González, “Pixelated phase computer holograms for the accurate encoding of scalar complex fields,” *J. Opt. Soc. Am. A* **24**, 3500–3507 (2007).
  - [3] L. Mandel and E. Wolf, *Optical Coherence and Quantum Optics* (Cambridge University Press, 1995).
  - [4] J. Ma, S. Masoodian, D. A. Starkey, and E. R. Fossum, “Photon-number-resolving megapixel image sensor at room temperature without avalanche gain,” *Optica* **4**, 1474–1481 (2017).
  - [5] T. Malhotra, W. E. Farriss, J. Hassett, A. F. Abouraddy, J. R. Fienup, and A. N. Vamivakas, “Interferometric spatial mode analyzer with a bucket detector,” *Optics express* **26**, 8719–8728 (2018).
